# Supplementary material for: Magnetic Induction in Convecting Galilean Oceans
Source: arXiv:2002.01636 source file (2020-03-06)
Supplement: Supplementary file 1 [file si_template_2019.pdf]

## Supporting Information for "Magnetic Induction in Conveecting Galilean Oceans"

S. D. Vance<sup>1</sup>, B. G. Bills<sup>1</sup>, C. J. Cochrane<sup>1</sup>, K. M. Soderlund<sup>2</sup>, N. Gómez-Pérez<sup>3</sup>,  
M. J. Styczinski<sup>4</sup>, and C. Paty<sup>5</sup>

<sup>1</sup>Jet Propulsion Laboratory, California Institute of Technology, Pasadena, USA

<sup>2</sup>Institute for Geophysics, John A. & Katherine G. Jackson School of Geosciences, The University of Texas at Austin, USA

<sup>3</sup>British Geological Survey, Edinburgh, UK

<sup>4</sup>Dept. of Physics, University of Washington, Seattle, USA

<sup>5</sup>Dept. of Earth Sciences, University of Oregon, Eugene, USA

### Contents of this file

1. Text S1
2. Figures S1 to S6

### Introduction

Text S1.

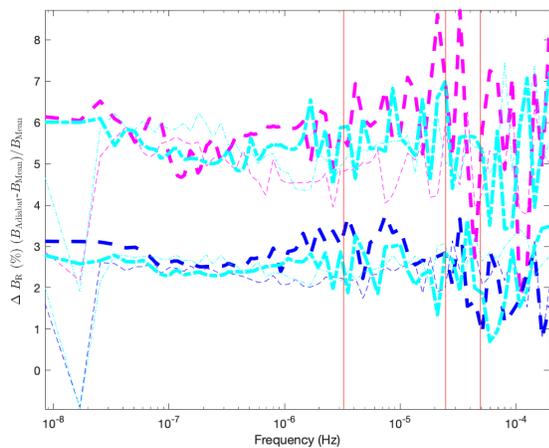

**Figure S1.** Europa: Differences (in %) from the nominal adiabatic case studied here, for oceans with the equivalent mean conductivity. Upper curves are for thinner ice (5 km) and lower curves for thicker ice (30 km). Thick lines are higher salinities (10wt% and 3.5wt%, respectively) for oceans with aqueous  $\text{MgSO}_4$  (--) and seawater (-.-.) Thinner lines are for oceans with 10% of those concentrations. Vertical lines are the strongest inducing frequencies shown in Figure 1.

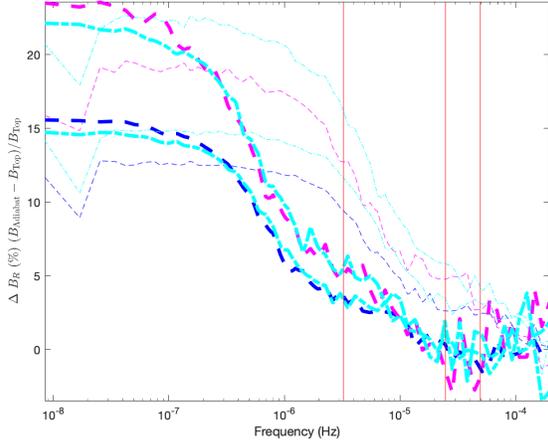

**Figure S2.** Europa: Differences (in %) from the nominal adiabatic case studied here with the conductivity at the top of the ocean (b). Upper curves are for thinner ice (5 km) and lower curves for thicker ice (30 km). Thick lines are higher salinities (10wt% and 3.5wt%, respectively) for oceans with aqueous  $\text{MgSO}_4$  (—) and seawater (---). Thinner lines are for oceans with 10% of those concentrations. Vertical lines are the strongest inducing frequencies shown in Figure 1.

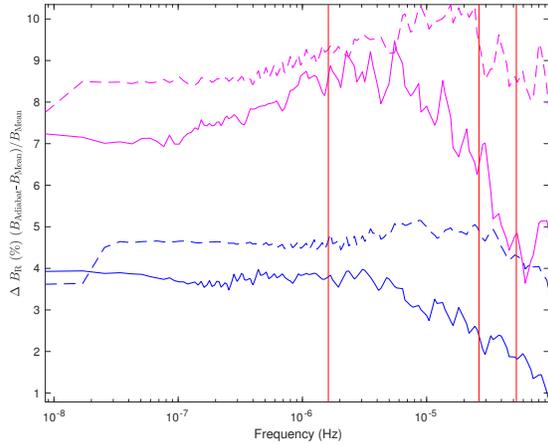

**Figure S3.** Ganymede: Differences (in %) from the nominal adiabatic case studied here for oceans with the thinner mean conductivity. Upper curves are for thinner ice ( $\sim 30$  km) and lower curves for thicker ice ( $\sim 100$  km). Thick lines are higher salinity (10wt%) for oceans with aqueous  $\text{MgSO}_4$  (—). Thinner lines are for oceans with 1wt%. Vertical lines are the strongest inducing frequencies shown in Figure 1.

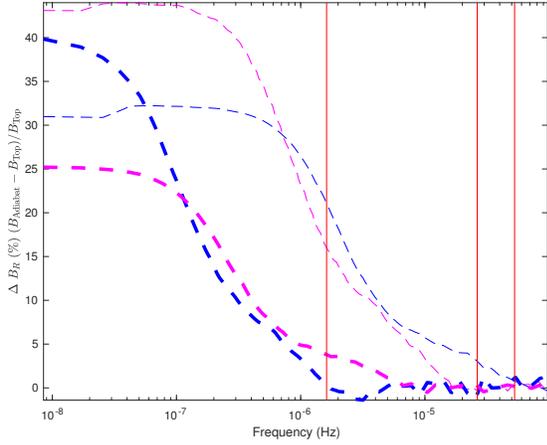

**Figure S4.** Ganymede: Differences (in %) from the nominal adiabatic case studied here with the conductivity at the top of the ocean (b). Upper curves are for thinner ice ( $\sim 30$  km) and lower curves for thicker ice ( $\sim 100$  km). Thick lines are higher salinity (10wt%) for oceans with aqueous  $\text{MgSO}_4$  (—). Thinner lines are for oceans with 1wt%. Vertical lines are the strongest inducing frequencies shown in Figure 1.

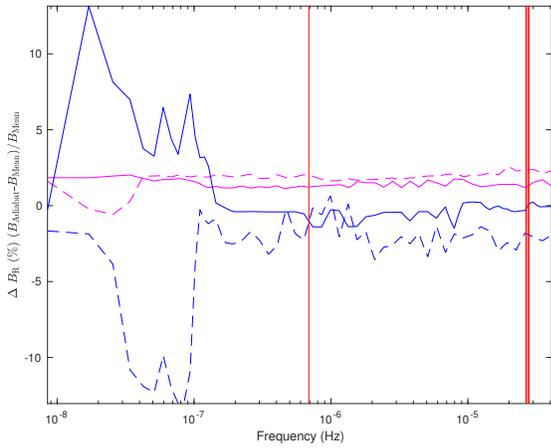

**Figure S5.** Callisto: Differences (in %) from the nominal adiabatic case studied here, for oceans with the equivalent mean conductivity (a) and with the conductivity at the top of the ocean (b). Upper curves are for thinner ice ( $\sim 30$  km) and lower curves for thicker ice ( $\sim 100$  km). Thick lines are higher salinity (10wt%) for oceans with aqueous  $\text{MgSO}_4$  (—). Thinner lines are for oceans with 1wt%. Vertical lines are the strongest inducing frequencies shown in Figure 1.

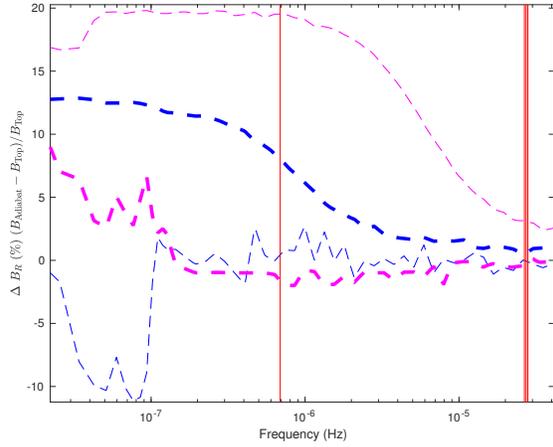

**Figure S6.** Callisto: Differences (in %) from the nominal adiabatic case studied here with the conductivity at the top of the ocean (b). Upper curves are for thinner ice ( $\sim 30$  km) and lower curves for thicker ice ( $\sim 100$  km). Thick lines are higher salinity (10wt%) for oceans with aqueous  $\text{MgSO}_4$  (—). Thinner lines are for oceans with 1wt%. Vertical lines are the strongest inducing frequencies shown in Figure 1.
